# Supplementary material for: Task-Guided IRL in POMDPs that Scales
Source: arXiv:2301.01219 source file (2022-12-30)
Supplement: Supplementary file 2 [file avoid_mem1_trajsize10pomdp_irl_si.tex]

% $\mathrm{Guided \ policy, \ |n|=1}$
x	y	err
0	0.0	0.0
1	0.0	0.0
2	-0.09999999999999991	9.71445146547012e-17
3	-0.09999999999999991	9.71445146547012e-17
4	-0.19999999999999982	1.942890293094024e-16
5	-0.19999999999999982	1.942890293094024e-16
6	-0.29999999999998495	1.509903313490213e-14
7	-0.29999999999998495	1.509903313490213e-14
8	-0.39999999999999963	3.885780586188048e-16
9	-0.39999999999999963	3.885780586188048e-16
10	-0.5	0.0
11	-0.5	0.0
12	-0.5999999999999699	3.008704396734174e-14
13	-0.5999999999999699	3.008704396734174e-14
14	-0.7000000000000268	2.6867397195928788e-14
15	-0.7000000000000268	2.6867397195928788e-14
16	-0.7999999999999993	6.661338147750939e-16
17	-0.7999999999999993	6.661338147750939e-16
18	-0.899966666666717	0.001825437542679066
19	-0.899966666666717	0.001825437542679066
20	-0.9998	0.005160103358138086
21	4.5002	15.644418385695033
22	4.41136666666648	15.675650570195678
23	4.41136666666648	15.675650570195678
24	4.322533333333139	15.706883806648365
25	4.322533333333139	15.706883806648365
26	4.233700000000191	15.738118088788697
27	4.233700000000191	15.738118088788697
28	4.14486666666685	15.769353410403717
29	4.14486666666685	15.769353410403717
30	4.0560333333333345	15.800589765329248
31	4.0560333333333345	15.800589765329248
32	3.96723333333316	15.831815531146043
33	7.083900000000166	19.027971098447182
34	7.001333333333025	19.06565301501351
35	7.001333333333025	19.06565301501351
36	6.918766666666995	19.103335951578668
37	7.218766666667004	19.355004119836376
38	7.136799999999856	19.393198268808884
39	7.136799999999856	19.393198268808884
40	7.054833333333347	19.43139341303707
41	7.054833333333347	19.43139341303707
42	6.972866666666823	19.469589546664153
43	6.972866666666823	19.469589546664153
44	6.890933333333033	19.507771215481
45	8.624266666666342	20.801445249362192
46	8.545866666667006	20.84224227177915
47	8.545866666667006	20.84224227177915
48	8.467533333333035	20.88300615130768
49	9.250866666666303	21.39222286834397
50	9.174100000000003	21.4340331993303
51	9.174100000000003	21.4340331993303
52	9.09733333333369	21.47584518062564
53	9.09733333333369	21.47584518062564
54	9.020599999999657	21.5176407235239
55	9.020599999999657	21.5176407235239
56	8.943866666667017	21.559438050396036
57	9.760533333333704	22.040737488771008
58	9.685433333332977	22.08353620110542
59	9.685433333332977	22.08353620110542
60	9.610333333333344	22.12633664261285
61	10.843666666666682	22.77311660464819
62	10.771033333333731	22.817270891415472
63	10.771033333333731	22.817270891415472
64	10.69839999999966	22.861426846109396
65	10.74839999999966	22.88563954623108
66	10.675866666667037	22.929848180531607
67	10.675866666667037	22.929848180531607
68	10.603333333332975	22.974058462148292
69	10.903333333332967	23.115262538466354
70	10.831433333333345	23.159753926705942
71	10.831433333333345	23.159753926705942
72	10.759533333333719	23.204247077828462
73	12.042866666667125	23.750803546734346
74	11.973533333333219	23.796469055630254
75	11.973533333333219	23.796469055630254
76	11.90420000000021	23.8421362792848
77	11.97086666666687	23.868021659022666
78	11.901666666666305	23.913746616167142
79	11.901666666666305	23.913746616167142
80	11.832466666666711	23.959473267350138
81	11.999133333333377	24.022581583075898
82	11.930266666667114	24.06844789197843
83	11.930266666667114	24.06844789197843
84	11.861466666666544	24.11427160795535
85	12.9781333333334	24.499262747728633
86	12.911566666666724	24.54593821549486
87	12.911566666666724	24.54593821549486
88	12.845066666666261	24.592568979176168
89	13.061733333332924	24.65984541034743
90	12.995666666666715	24.706628555016593
91	12.995666666666715	24.706628555016593
92	12.9296000000005	24.753413848867844
93	12.962933333333837	24.763449128279575
94	12.896933333333374	24.81025924751486
95	12.896933333333374	24.81025924751486
96	12.8309333333334	24.85707149140673
97	13.630933333333296	25.080361037982797
98	13.56656666666625	25.127663617592287
99	13.56656666666625	25.127663617592287
100	13.50220000000005	25.17496842421108
101	13.768866666666714	25.242294217883785
102	13.705033333333855	25.28975849361854
103	13.705033333333855	25.28975849361854
104	13.641200000000145	25.337224970913002
105	13.857866666666835	25.388911715856302
106	13.794466666666594	25.436503219760127
107	13.794466666666594	25.436503219760127
108	13.731099999999579	25.484071942882238
109	14.097766666666235	25.565745409543197
110	14.035133333333373	25.6135139912947
111	14.035133333333373	25.6135139912947
112	13.972500000000506	25.661284855140078
113	14.689166666667184	25.80246782717225
114	14.627966666666905	25.850592150513616
115	14.627966666666905	25.850592150513616
116	14.566766666666528	25.898718736883872
117	14.683433333333184	25.919319220976952
118	14.62246666666625	25.96750087928256
119	14.62246666666625	25.96750087928256
120	14.561500000000049	26.015684777008474
121	14.928166666666716	26.075588391678895
122	14.867933333333855	26.123932547166685
123	14.867933333333855	26.123932547166685
124	14.807700000000274	26.172278923382233
125	15.407700000000336	26.25678853255576
126	15.348666666666452	26.305370393810275
127	15.348666666666452	26.305370393810275
128	15.289666666666248	26.353927092982467
129	15.556333333332907	26.386054521702047
130	15.497866666666724	26.434706897981602
131	15.497866666666724	26.434706897981602
132	15.43940000000054	26.483361587482552
133	15.656066666667211	26.50668638656179
134	15.59803333333368	26.55541462926616
135	15.59803333333368	26.55541462926616
136	15.540033333333117	26.604117237729913
137	15.940033333333083	26.64107781851554
138	15.882833333332911	26.689903246462446
139	15.882833333332911	26.689903246462446
140	15.82563333333339	26.73873107682698
141	16.108966666666728	26.760261637963158
142	16.052333333333866	26.809168852382612
143	16.052333333333866	26.809168852382612
144	15.995700000000364	26.85807845279784
145	16.229033333333703	26.872736005083294
146	16.172866666666433	26.921706182599337
147	16.172866666666433	26.921706182599337
148	16.1166999999996	26.97067872913105
149	16.48336666666626	26.98834600339393
150	16.427933333333392	27.037402976781756
151	16.427933333333392	27.037402976781756
152	16.37256666666719	27.086403429498887
153	16.572566666667193	27.093250526263375
154	16.517600000000368	27.142293017355595
155	16.517600000000368	27.142293017355595
156	16.462633333333095	27.191338088913206
157	16.59596666666642	27.19462668246992
158	16.541266666666267	27.243698667071822
159	16.541266666666267	27.243698667071822
160	16.486566666666725	27.29277321097185
161	16.836566666666727	27.297112903728237
162	16.78260000000052	27.346216384965032
163	16.78260000000052	27.346216384965032
164	16.728633333333704	27.395322535039845
165	17.228633333333764	27.392062052090175
166	17.175666666666388	27.441233473653007
167	17.175666666666388	27.441233473653007
168	17.122699999999607	27.49040756415433
169	17.339366666666272	27.48543360155583
170	17.2868333333334	27.534630981830112
171	17.2868333333334	27.534630981830112
172	17.234300000000527	27.58383101583205
173	17.650966666667216	27.568077052977493
174	17.599266666667127	27.61730833122985
175	17.599266666667127	27.61730833122985
176	17.547566666666366	27.666542262189907
177	17.930899999999692	27.645207213126344
178	17.879966666666288	27.69445736362363
179	17.879966666666288	27.69445736362363
180	17.829066666666744	27.743677990890898
181	18.04573333333341	27.728543569077576
182	17.9952666666672	27.777768885607607
183	17.9952666666672	27.777768885607607
184	17.94480000000046	27.826996956672467
185	18.111466666667127	27.813648601281198
186	18.06133333333303	27.862878139600493
187	18.06133333333303	27.862878139600493
188	18.01119999999963	27.912110416328684
189	18.294533333332964	27.88618445483127
190	18.24496666666674	27.935411839912568
191	18.24496666666674	27.935411839912568
192	18.195400000000518	27.984641957807433
193	18.362066666667186	27.967491981386573
194	18.31283333333379	28.016717128151953
195	18.31283333333379	28.016717128151953
196	18.263599999999702	28.065944993413765
197	18.563599999999692	28.03157341950932
198	18.514999999999628	28.08075049448135
199	18.514999999999628	28.08075049448135
200	18.466400000000075	28.129930401146016
201	18.74973333333341	28.093565335538948
202	18.701700000000525	28.14272197999519
203	18.701700000000525	28.14272197999519
204	18.65366666666714	28.19188145351235
205	18.787000000000475	28.173334159567414
206	18.739266666666346	28.222447533754863
207	18.739266666666346	28.222447533754863
208	18.691533333332963	28.271563834511877
209	18.858199999999627	28.24694141719867
210	18.81080000000007	28.296039829393973
211	18.81080000000007	28.296039829393973
212	18.76340000000052	28.345141155172644
213	19.14673333333386	28.283472370429845
214	19.100100000000495	28.33251977245703
215	19.100100000000495	28.33251977245703
216	19.053466666666335	28.381570099548235
217	19.336799999999652	28.331659777711227
218	19.29073333333297	28.380663031876058
219	19.29073333333297	28.380663031876058
220	19.24466666666674	28.429669212911435
221	19.528000000000077	28.375937623275203
222	19.482533333333844	28.42485405853312
223	19.482533333333844	28.42485405853312
224	19.437100000000502	28.47373772894409
225	19.603766666667173	28.44023433703668
226	19.558666666666323	28.489083960157664
227	19.558666666666323	28.489083960157664
228	19.513566666666318	28.5379367266142
229	19.730233333332986	28.492180376591115
230	19.685566666666745	28.540984245097246
231	19.685566666666745	28.540984245097246
232	19.640933333333837	28.589754886360808
233	19.874266666667175	28.537820597624645
234	19.83010000000051	28.58653349609447
235	19.83010000000051	28.58653349609447
236	19.785933333332988	28.63524964320869
237	19.919266666666317	28.6042565969159
238	19.875366666666327	28.652938939410035
239	19.875366666666327	28.652938939410035
240	19.831466666666746	28.701624515850995
241	20.048133333333418	28.649188525720053
242	20.0047000000005	28.697776474435525
243	20.0047000000005	28.697776474435525
244	19.961266666667168	28.746367765839572
245	20.161266666667178	28.69580375354938
246	20.11823333333299	28.744335631196652
247	20.11823333333299	28.744335631196652
248	20.075199999999672	28.792870847254168
249	20.341866666666334	28.722317580275963
250	20.299366666666742	28.770766927540954
251	20.299366666666742	28.770766927540954
252	20.256900000000492	28.8191816745379
253	20.45690000000049	28.763909198681567
254	20.41483333333383	28.81225601439256
255	20.41483333333383	28.81225601439256
256	20.372766666666333	28.860606282824552
257	20.522766666666328	28.81770749057312
258	20.480999999999682	28.86600524838869
259	20.480999999999682	28.86600524838869
260	20.439233333333416	28.914306448749574
261	20.539233333333417	28.884931551685458
262	20.49766666666715	28.933197678253386
263	20.49766666666715	28.933197678253386
264	20.456133333333835	28.981428577319026
265	20.65613333333385	28.920939629425884
266	20.615033333333	28.969054937966252
267	20.615033333333	28.969054937966252
268	20.573966666666358	29.01713491942697
269	20.75729999999969	28.95980064462902
270	20.71663333333342	29.00776781023024
271	20.71663333333342	29.00776781023024
272	20.675966666667154	29.05573883186488
273	20.89263333333383	28.985676274076297
274	20.85240000000052	29.033555429995992
275	20.85240000000052	29.033555429995992
276	20.81216666666633	29.081438444001403
277	20.978833333332993	29.025820033874925
278	20.93896666666636	29.073590391720593
279	20.93896666666636	29.073590391720593
280	20.89910000000009	29.12136470914977
281	21.132433333333427	29.041003048773845
282	21.093033333333818	29.088669296919516
283	21.093033333333818	29.088669296919516
284	21.053633333333856	29.136339511548407
285	21.336966666667195	29.035075514491787
286	21.298133333333006	29.082606884222443
287	21.298133333333006	29.082606884222443
288	21.259299999999715	29.130142238638456
289	21.475966666666377	29.049943414727764
290	21.43756666666676	29.097368473435488
291	21.43756666666676	29.097368473435488
292	21.399200000000484	29.1447564070566
293	21.682533333333815	29.036247489110593
294	21.644733333333875	29.083482922939165
295	21.644733333333875	29.083482922939165
296	21.606933333332996	29.130722475230293
297	21.69026666666633	29.09795339759952
298	21.652633333333053	29.145149506088323
299	21.652633333333053	29.145149506088323
