# Supplementary material for: Task-Guided IRL in POMDPs that Scales
Source: arXiv:2301.01219 source file (2022-12-30)
Supplement: Supplementary file 4 [file evade_mem1_trajsize10pomdp_irl_si.tex]

% $\mathrm{Guided \ policy, \ |n|=1}$
x	y	err
0	0.0	0.0
1	0.0	0.0
2	-0.09999999999999991	9.71445146547012e-17
3	-0.09999999999999991	9.71445146547012e-17
4	-0.19999999999999982	1.942890293094024e-16
5	-0.19999999999999982	1.942890293094024e-16
6	-0.29999999999998495	1.509903313490213e-14
7	-0.29999999999998495	1.509903313490213e-14
8	-0.3999666666666663	0.0018254375426790712
9	-0.40069999999999983	0.008727924533740187
10	-0.49973333333333336	0.0057673410010352175
11	-0.5006333333333333	0.011087480427140296
12	-0.59939999999997	0.01093800713110013
13	-0.6468999999999975	0.05167581639413256
14	-0.6995000000000267	0.017974519001445054
15	-0.7500333333333336	0.05360347210976373
16	-0.7990999999999996	0.02413552015874765
17	-0.10393333333332855	3.8194970692778383
18	3.6960000000001862	8.424015511223528
19	6.2686000000000455	9.62765984234989
20	7.026033333333317	9.84855178518928
21	7.819633333333373	10.001194488604245
22	8.723333333333377	10.08981675860479
23	9.394966666666557	10.09958867143714
24	9.889699999999763	10.083994111627367
25	10.408933333333259	10.034378582099148
26	10.980999999999973	9.942573727829952
27	11.597133333333096	9.79740706082769
28	11.958899999999675	9.698478959266486
29	12.303066666666433	9.587873100722414
30	12.766566666666536	9.408827355851464
31	13.200033333333248	9.21294940100916
32	13.485399999999924	9.074690821546794
33	13.713866666666553	8.954759314589152
34	13.940266666666485	8.829181082951779
35	14.190499999999757	8.674053248049473
36	14.538699999999697	8.436559269631195
37	14.763666666666344	8.271491998961709
38	14.97339999999969	8.110805083754965
39	15.232433333333075	7.891714098484621
40	15.403999999999792	7.741885472329448
41	15.543833333333144	7.613786747662892
42	15.70993333333316	7.452853681346173
43	15.883766666666473	7.273513580947101
44	16.02396666666643	7.123517080690516
45	16.17189999999972	6.95574825042803
46	16.29289999999968	6.813940582120239
47	16.41476666666635	6.6635444981547955
48	16.522966666666374	6.5260423840860815
49	16.632299999999738	6.3788400233375375
50	16.734466666666428	6.2364048443171285
51	16.844399999999773	6.07445212673545
52	16.940499999999773	5.928641475920123
53	17.044033333333097	5.7628006269135685
54	17.147499999999727	5.589548021381806
55	17.21129999999971	5.479941208017984
56	17.248633333333032	5.415878949800168
57	17.299366666666376	5.324488357162189
58	17.383766666666386	5.163360644537224
59	17.46163333333306	5.0077131839016165
60	17.553199999999734	4.815023339507306
61	17.611466666666406	4.687821297314504
62	17.656633333333076	4.585507169211408
63	17.701999999999728	4.479785262710762
64	17.72059999999972	4.437274949034946
65	17.75279999999972	4.3595151290023
66	17.791433333333046	4.263025914248719
67	17.810599999999713	4.214508390468991
68	17.842699999999716	4.130801380281271
69	17.875299999999726	4.041653940735994
70	17.88086666666639	4.0285390961102685
71	17.880166666666394	4.032276855436464
72	17.92596666666639	3.901330849708721
73	17.95196666666639	3.8245561135320774
74	17.96446666666639	3.7886572883924305
75	17.963966666666387	3.79153683865644
76	17.97649999999972	3.7545800142404318
77	17.975999999999722	3.7575014748278366
78	17.981866666666388	3.7410717513686964
79	17.99476666666639	3.7003201589712407
80	18.014166666666387	3.638140913372585
81	18.013699999999726	3.640982785366224
82	18.026499999999725	3.599435291357066
83	18.032733333333052	3.579225502193933
84	18.038966666666386	3.558896589144238
85	18.05189999999972	3.5146981458820075
86	18.05149999999972	3.5172571344728243
87	18.064533333333053	3.472038130870988
88	18.064099999999723	3.4748584417210413
89	18.06379999999972	3.476811215275678
90	18.070033333333054	3.4554795131147102
91	18.076433333333057	3.4329027482422
92	18.076066666666385	3.4353418843285812
93	18.075799999999713	3.437114248901281
94	18.075399999999714	3.439783157894306
95	18.095166666666383	3.3646307334122625
96	18.101499999999717	3.34107883025829
97	18.10803333333305	3.3159541812609663
98	18.107699999999717	3.318283297630465
99	18.107566666666383	3.3192126695280324
100	18.107199999999715	3.321782878716392
101	18.113766666666383	3.2958681929888702
102	18.11343333333305	3.2982332966133128
103	18.119999999999713	3.2719189069005505
104	18.119699999999714	3.2740742065505595
105	18.126199999999713	3.2472173051193916
106	18.132699999999712	3.2203354964972095
107	18.13916666666638	3.193252673824741
108	18.145699999999714	3.165852414437504
109	18.145533333333045	3.1671017322185984
110	18.145399999999714	3.1681044027409597
111	18.14526666666638	3.1691088540611503
112	18.158466666666378	3.110881169200904
113	18.15839999999971	3.111394559786109
114	18.15826666666638	3.112424295554093
115	18.164866666666377	3.0828967409817003
116	18.171433333333045	3.0533337974890182
117	18.17139999999971	3.0535993035541877
118	18.17129999999971	3.054394589767368
119	18.171266666666376	3.0546610934039373
120	18.177833333333044	3.02371272426615
