# Supplementary material for: Task-Guided IRL in POMDPs that Scales
Source: arXiv:2301.01219 source file (2022-12-30)
Supplement: Supplementary file 5 [file intercept_mem1_trajsize10mdp_irl_si.tex]

% $\mathrm{Guided \ policy, \ |n|=1}$
x	y	err
0	0.0	0.0
1	-0.09999999999999991	9.71445146547012e-17
2	-0.19999999999999982	1.942890293094024e-16
3	-0.29999999999998495	1.509903313490213e-14
4	-0.39999999999999963	3.885780586188048e-16
5	3.3458000000000356	7.906352026061179
6	4.2163333333332025	8.602193124753263
7	8.213799999999756	10.029156306821731
8	9.712333333333513	10.127253718994432
9	13.550199999999784	9.191212830379428
10	14.660666666666591	8.591931072556164
11	16.996199999999977	6.492225521858224
12	17.514366666666632	5.801808648937762
13	18.102166666666538	4.81477780438047
14	18.391666666666538	4.210875271906718
15	18.80323333333321	3.0883241753776827
16	18.888566666666563	2.7926413922227344
17	18.994433333333227	2.3628243718529394
18	19.02716666666654	2.2121931739540663
19	19.08016666666654	1.9364942479187128
20	19.099933333333208	1.8221489132950408
21	19.119799999999877	1.697490685295986
22	19.119666666666546	1.6991605443734747
23	19.14633333333321	1.5108672638219722
24	19.14633333333321	1.5108672638219722
25	19.14633333333321	1.5108672638219722
26	19.14633333333321	1.5108672638219722
27	19.14633333333321	1.5108672638219722
28	19.14633333333321	1.5108672638219722
29	19.14633333333321	1.5108672638219722
30	19.14633333333321	1.5108672638219722
31	19.14633333333321	1.5108672638219722
32	19.14633333333321	1.5108672638219722
33	19.14633333333321	1.5108672638219722
34	19.14633333333321	1.5108672638219722
35	19.14633333333321	1.5108672638219722
36	19.14633333333321	1.5108672638219722
37	19.14633333333321	1.5108672638219722
38	19.14633333333321	1.5108672638219722
39	19.14633333333321	1.5108672638219722
40	19.14633333333321	1.5108672638219722
41	19.14633333333321	1.5108672638219722
42	19.14633333333321	1.5108672638219722
43	19.14633333333321	1.5108672638219722
44	19.14633333333321	1.5108672638219722
45	19.14633333333321	1.5108672638219722
46	19.14633333333321	1.5108672638219722
47	19.14633333333321	1.5108672638219722
48	19.14633333333321	1.5108672638219722
49	19.14633333333321	1.5108672638219722
50	19.14633333333321	1.5108672638219722
51	19.14633333333321	1.5108672638219722
52	19.14633333333321	1.5108672638219722
53	19.14633333333321	1.5108672638219722
54	19.14633333333321	1.5108672638219722
55	19.14633333333321	1.5108672638219722
56	19.14633333333321	1.5108672638219722
57	19.14633333333321	1.5108672638219722
58	19.14633333333321	1.5108672638219722
59	19.14633333333321	1.5108672638219722
60	19.14633333333321	1.5108672638219722
61	19.14633333333321	1.5108672638219722
62	19.14633333333321	1.5108672638219722
63	19.14633333333321	1.5108672638219722
64	19.14633333333321	1.5108672638219722
65	19.14633333333321	1.5108672638219722
66	19.14633333333321	1.5108672638219722
67	19.14633333333321	1.5108672638219722
68	19.14633333333321	1.5108672638219722
69	19.14633333333321	1.5108672638219722
70	19.14633333333321	1.5108672638219722
71	19.14633333333321	1.5108672638219722
72	19.14633333333321	1.5108672638219722
73	19.14633333333321	1.5108672638219722
74	19.14633333333321	1.5108672638219722
75	19.14633333333321	1.5108672638219722
76	19.14633333333321	1.5108672638219722
77	19.14633333333321	1.5108672638219722
78	19.14633333333321	1.5108672638219722
79	19.14633333333321	1.5108672638219722
80	19.14633333333321	1.5108672638219722
81	19.14633333333321	1.5108672638219722
82	19.14633333333321	1.5108672638219722
83	19.14633333333321	1.5108672638219722
84	19.14633333333321	1.5108672638219722
85	19.14633333333321	1.5108672638219722
86	19.14633333333321	1.5108672638219722
87	19.14633333333321	1.5108672638219722
88	19.14633333333321	1.5108672638219722
89	19.14633333333321	1.5108672638219722
90	19.14633333333321	1.5108672638219722
91	19.14633333333321	1.5108672638219722
92	19.14633333333321	1.5108672638219722
93	19.14633333333321	1.5108672638219722
94	19.14633333333321	1.5108672638219722
95	19.14633333333321	1.5108672638219722
96	19.14633333333321	1.5108672638219722
97	19.14633333333321	1.5108672638219722
98	19.14633333333321	1.5108672638219722
99	19.14633333333321	1.5108672638219722
100	19.14633333333321	1.5108672638219722
101	19.14633333333321	1.5108672638219722
102	19.14633333333321	1.5108672638219722
103	19.14633333333321	1.5108672638219722
104	19.14633333333321	1.5108672638219722
105	19.14633333333321	1.5108672638219722
106	19.14633333333321	1.5108672638219722
107	19.14633333333321	1.5108672638219722
108	19.14633333333321	1.5108672638219722
109	19.14633333333321	1.5108672638219722
110	19.14633333333321	1.5108672638219722
111	19.14633333333321	1.5108672638219722
112	19.14633333333321	1.5108672638219722
113	19.14633333333321	1.5108672638219722
114	19.14633333333321	1.5108672638219722
115	19.14633333333321	1.5108672638219722
116	19.14633333333321	1.5108672638219722
117	19.14633333333321	1.5108672638219722
118	19.14633333333321	1.5108672638219722
119	19.14633333333321	1.5108672638219722
120	19.14633333333321	1.5108672638219722
