# Supplementary material for: Task-Guided IRL in POMDPs that Scales
Source: arXiv:2301.01219 source file (2022-12-30)
Supplement: Supplementary file 6 [file intercept_mem1_trajsize10pomdp_irl_si.tex]

% $\mathrm{Guided \ policy, \ |n|=1}$
x	y	err
0	0.0	0.0
1	-0.09999999999999991	9.71445146547012e-17
2	-0.19999999999999982	1.942890293094024e-16
3	-0.29999999999998495	1.509903313490213e-14
4	-0.39999999999999963	3.885780586188048e-16
5	3.272100000000034	7.8479597087395065
6	4.1154666666665385	8.539574976673016
7	8.259833333333084	10.033388425928468
8	9.751900000000179	10.124725990860114
9	13.57656666666645	9.178046317829267
10	14.714033333333255	8.556385514079903
11	17.00299999999999	6.483492191712834
12	17.548066666666635	5.750772376723747
13	18.18299999999988	4.654159895548676
14	18.399366666666538	4.193305330987572
15	18.831233333333213	2.9937837506332436
16	18.903466666666557	2.7362592437283575
17	19.00956666666655	2.293122720706883
18	19.03579999999987	2.1689947809987906
19	19.082266666666538	1.9233804084360167
20	19.102166666666538	1.806630004240549
21	19.122166666666537	1.6791144408751748
22	19.122166666666537	1.6791144408751748
23	19.122166666666537	1.6791144408751748
24	19.122166666666537	1.6791144408751748
25	19.122166666666537	1.6791144408751748
26	19.122166666666537	1.6791144408751748
27	19.122166666666537	1.6791144408751748
28	19.122166666666537	1.6791144408751748
29	19.122166666666537	1.6791144408751748
30	19.122166666666537	1.6791144408751748
31	19.122166666666537	1.6791144408751748
32	19.122166666666537	1.6791144408751748
33	19.122166666666537	1.6791144408751748
34	19.122166666666537	1.6791144408751748
35	19.122166666666537	1.6791144408751748
36	19.122166666666537	1.6791144408751748
37	19.122166666666537	1.6791144408751748
38	19.122166666666537	1.6791144408751748
39	19.122166666666537	1.6791144408751748
40	19.122166666666537	1.6791144408751748
41	19.122166666666537	1.6791144408751748
42	19.122166666666537	1.6791144408751748
43	19.122166666666537	1.6791144408751748
44	19.122166666666537	1.6791144408751748
45	19.122166666666537	1.6791144408751748
46	19.122166666666537	1.6791144408751748
47	19.122166666666537	1.6791144408751748
48	19.122166666666537	1.6791144408751748
49	19.122166666666537	1.6791144408751748
50	19.122166666666537	1.6791144408751748
51	19.122166666666537	1.6791144408751748
52	19.122166666666537	1.6791144408751748
53	19.122166666666537	1.6791144408751748
54	19.122166666666537	1.6791144408751748
55	19.122166666666537	1.6791144408751748
56	19.122166666666537	1.6791144408751748
57	19.122166666666537	1.6791144408751748
58	19.122166666666537	1.6791144408751748
59	19.122166666666537	1.6791144408751748
60	19.122166666666537	1.6791144408751748
61	19.122166666666537	1.6791144408751748
62	19.122166666666537	1.6791144408751748
63	19.122166666666537	1.6791144408751748
64	19.122166666666537	1.6791144408751748
65	19.122166666666537	1.6791144408751748
66	19.122166666666537	1.6791144408751748
67	19.122166666666537	1.6791144408751748
68	19.122166666666537	1.6791144408751748
69	19.122166666666537	1.6791144408751748
70	19.122166666666537	1.6791144408751748
71	19.122166666666537	1.6791144408751748
72	19.122166666666537	1.6791144408751748
73	19.122166666666537	1.6791144408751748
74	19.122166666666537	1.6791144408751748
75	19.122166666666537	1.6791144408751748
76	19.122166666666537	1.6791144408751748
77	19.122166666666537	1.6791144408751748
78	19.122166666666537	1.6791144408751748
79	19.122166666666537	1.6791144408751748
80	19.122166666666537	1.6791144408751748
81	19.122166666666537	1.6791144408751748
82	19.122166666666537	1.6791144408751748
83	19.122166666666537	1.6791144408751748
84	19.122166666666537	1.6791144408751748
85	19.122166666666537	1.6791144408751748
86	19.122166666666537	1.6791144408751748
87	19.122166666666537	1.6791144408751748
88	19.122166666666537	1.6791144408751748
89	19.122166666666537	1.6791144408751748
90	19.122166666666537	1.6791144408751748
91	19.122166666666537	1.6791144408751748
92	19.122166666666537	1.6791144408751748
93	19.122166666666537	1.6791144408751748
94	19.122166666666537	1.6791144408751748
95	19.122166666666537	1.6791144408751748
96	19.122166666666537	1.6791144408751748
97	19.122166666666537	1.6791144408751748
98	19.122166666666537	1.6791144408751748
99	19.122166666666537	1.6791144408751748
100	19.122166666666537	1.6791144408751748
101	19.122166666666537	1.6791144408751748
102	19.122166666666537	1.6791144408751748
103	19.122166666666537	1.6791144408751748
104	19.122166666666537	1.6791144408751748
105	19.122166666666537	1.6791144408751748
106	19.122166666666537	1.6791144408751748
107	19.122166666666537	1.6791144408751748
108	19.122166666666537	1.6791144408751748
109	19.122166666666537	1.6791144408751748
110	19.122166666666537	1.6791144408751748
111	19.122166666666537	1.6791144408751748
112	19.122166666666537	1.6791144408751748
113	19.122166666666537	1.6791144408751748
114	19.122166666666537	1.6791144408751748
115	19.122166666666537	1.6791144408751748
116	19.122166666666537	1.6791144408751748
117	19.122166666666537	1.6791144408751748
118	19.122166666666537	1.6791144408751748
119	19.122166666666537	1.6791144408751748
