# Supplementary material for: Task-Guided IRL in POMDPs that Scales
Source: arXiv:2301.01219 source file (2022-12-30)
Supplement: Supplementary file 10 [file maze_mem1_trajsize5pomdp_irl_si.tex]

% $\mathrm{Guided \ policy, \ |n|=1}$
x	y	err
0	0.0	0.0
1	-0.09999999999999647	3.5388358909926865e-15
2	0.7749999999999734	9.555070643380835
3	1.0622500000000208	11.859932543547425
4	1.5385499999999601	13.773174249152072
5	2.3727500000000004	15.989394686401003
6	3.165049999999933	17.65174533856342
7	4.474700000000039	19.69769453286341
8	5.868150000000125	21.588139117985442
9	6.75015000000018	22.834502621636375
10	8.539699999999996	24.465228670707436
11	9.748250000000017	25.556585392761402
12	11.304749999999693	26.598216339399713
13	12.324700000000247	27.403619832241272
14	13.677099999999724	28.142140387504167
15	14.662499999999959	28.685982007767947
16	15.945150000000268	29.186879697519895
17	17.245699999999804	29.61576896705569
18	18.324200000000065	29.93513628430656
19	19.320099999999655	30.190372571235244
20	20.36324999999998	30.42804831791729
21	21.24375000000033	30.59354688390184
22	22.40135000000021	30.61751726018152
23	23.36644999999981	30.676455293881368
24	24.33864999999972	30.681788917491353
25	24.923000000000005	30.622464156236823
26	25.723650000000273	30.563618170587965
27	26.301100000000226	30.52759536534107
28	26.94494999999982	30.32085807653692
29	27.815199999999763	30.159484229011507
30	28.52229999999999	29.990054229860874
31	29.090950000000213	29.769024389413644
32	29.545800000000206	29.580852461685403
33	30.221649999999826	29.06324958220427
34	30.793899999999823	28.7970875747878
35	31.362350000000003	28.33555588792106
36	31.71200000000017	28.02928407933383
37	32.02740000000019	27.79276775062173
38	32.523499999999856	27.531100373032718
39	32.8656999999999	27.17303559615671
40	33.23870000000002	26.869289575833537
41	33.57750000000013	26.604513033506045
42	33.812000000000175	26.41252403690336
43	34.066999999999915	26.30213453315146
44	34.25754999999997	26.098663816324063
45	34.513650000000055	25.833895538178144
46	34.755300000000084	25.61506006063624
47	34.962450000000175	25.315712018379077
48	35.10004999999996	25.22990239770056
49	35.21795000000004	25.130148284431176
50	35.56110000000007	24.818810140496378
51	35.57995000000008	24.81627375327528
52	35.76885000000014	24.702479322478915
53	35.93314999999998	24.45705820571029
54	35.99780000000005	24.391424828410447
55	36.087600000000066	24.309874870924386
56	36.18260000000008	24.211089344348004
57	36.24780000000014	23.98006724677811
58	36.28815000000001	23.95646623727093
59	36.45360000000005	23.833534925394478
60	36.54940000000008	23.696089965224203
61	36.615400000000086	23.6764482733369
62	36.631550000000125	23.695898792776386
63	36.747750000000025	23.588354010772022
64	36.81420000000006	23.496283501013504
65	36.900800000000075	23.449167988651496
66	36.97265000000009	23.397776325486618
67	37.05465000000012	23.264470730654903
68	37.101850000000056	23.16648897820937
69	37.22415000000009	23.027052172987798
70	37.34670000000009	22.676497284854246
71	37.36950000000011	22.660671211374094
72	37.42735000000013	22.63417254899101
73	37.45035000000008	22.617682902488013
74	37.558400000000084	22.492610996502865
75	37.70675000000009	22.27295556134156
76	37.72540000000011	22.272048061190947
77	37.794100000000114	22.094090277492803
78	37.79295000000009	22.09738842708564
79	37.8118000000001	22.091004521297787
80	37.83570000000011	22.04799300412624
81	37.85465000000011	22.04796063987546
82	37.87865000000012	22.015727768518072
83	37.87770000000009	22.01862649462956
84	37.95175000000011	21.903209968803715
85	38.00095000000012	21.82231092477376
86	38.000250000000115	21.824560131592616
87	37.98955000000013	21.86649550791113
88	38.013850000000105	21.809493189377488
89	38.01320000000011	21.811623409549235
90	38.05755000000011	21.788914910970206
91	38.08200000000012	21.650246095599037
92	38.076500000000124	21.670860106373272
93	38.07600000000011	21.67250571576798
94	38.07550000000012	21.674153495580846
95	38.125000000000114	21.60047349018068
96	38.124600000000115	21.60186554073514
97	38.14920000000012	21.542028209061563
98	38.173850000000115	21.493334808202842
99	38.17355000000012	21.494400559157278
