# Supplementary material for: Task-Guided IRL in POMDPs that Scales
Source: arXiv:2301.01219 source file (2022-12-30)
Supplement: Supplementary file 13 [file obstacle_mem5_trajsize10mdp_irl_si.tex]

% $\mathrm{Guided \ policy, \ |n|=10}$
x	y	err
0	0.0	0.0
1	-5.0	0.0
2	-10.0	0.0
3	-14.158333333333333	20.599351055042927
4	-14.941666666666666	50.33012613954132
5	-16.188333333333333	66.34816900680399
6	-14.368333333333334	87.88776553398118
7	-10.966666666666667	108.22891891213078
8	-4.285	130.52821064811718
9	6.8933333333333335	154.82236688828488
10	15.235	171.43391275259685
11	26.523333333333333	188.3514342628874
12	36.59166666666667	201.66500670804137
13	44.498333333333335	211.77060701906115
14	55.245	222.43706594975518
15	74.245	235.49332256987392
16	101.06	248.15648906822292
17	136.94166666666666	257.8363917885777
18	175.74166666666667	261.1097947809579
19	212.76833333333335	257.81743152320365
20	251.02666666666667	247.4124679333871
21	280.765	234.06973271869143
22	303.0683333333333	220.42457590724368
23	323.07666666666665	204.7181007846832
24	339.5883333333333	188.64885068266014
25	350.545	176.01594049498328
26	357.0733333333333	167.52308683349352
27	362.49	159.71359752173052
28	365.2683333333333	155.41322229427269
29	367.74	151.32611274991578
30	368.89	149.33982913699367
31	369.37833333333333	148.47700786279634
32	369.87333333333333	147.56716195986448
33	370.205	146.93927195160094
34	370.2033333333333	146.94537076372623
35	370.37	146.61575551988557
36	370.37	146.61575551988557
37	370.37	146.61575551988557
38	370.37	146.61575551988557
39	370.37	146.61575551988557
40	370.37	146.61575551988557
41	370.37	146.61575551988557
42	370.37	146.61575551988557
43	370.37	146.61575551988557
44	370.37	146.61575551988557
45	370.37	146.61575551988557
46	370.37	146.61575551988557
47	370.37	146.61575551988557
48	370.37	146.61575551988557
49	370.37	146.61575551988557
50	370.37	146.61575551988557
51	370.37	146.61575551988557
52	370.37	146.61575551988557
53	370.37	146.61575551988557
54	370.37	146.61575551988557
55	370.37	146.61575551988557
56	370.37	146.61575551988557
57	370.37	146.61575551988557
58	370.37	146.61575551988557
59	370.37	146.61575551988557
60	370.37	146.61575551988557
61	370.37	146.61575551988557
62	370.37	146.61575551988557
63	370.37	146.61575551988557
64	370.37	146.61575551988557
65	370.37	146.61575551988557
66	370.37	146.61575551988557
67	370.37	146.61575551988557
68	370.37	146.61575551988557
69	370.37	146.61575551988557
70	370.37	146.61575551988557
71	370.37	146.61575551988557
72	370.37	146.61575551988557
73	370.37	146.61575551988557
74	370.37	146.61575551988557
75	370.37	146.61575551988557
76	370.37	146.61575551988557
77	370.37	146.61575551988557
78	370.37	146.61575551988557
79	370.37	146.61575551988557
80	370.37	146.61575551988557
81	370.37	146.61575551988557
82	370.37	146.61575551988557
83	370.37	146.61575551988557
84	370.37	146.61575551988557
85	370.37	146.61575551988557
86	370.37	146.61575551988557
87	370.37	146.61575551988557
88	370.37	146.61575551988557
89	370.37	146.61575551988557
90	370.37	146.61575551988557
91	370.37	146.61575551988557
92	370.37	146.61575551988557
93	370.37	146.61575551988557
94	370.37	146.61575551988557
95	370.37	146.61575551988557
96	370.37	146.61575551988557
97	370.37	146.61575551988557
98	370.37	146.61575551988557
99	370.37	146.61575551988557
100	370.37	146.61575551988557
101	370.37	146.61575551988557
102	370.37	146.61575551988557
103	370.37	146.61575551988557
104	370.37	146.61575551988557
105	370.37	146.61575551988557
106	370.37	146.61575551988557
107	370.37	146.61575551988557
108	370.37	146.61575551988557
109	370.37	146.61575551988557
110	370.37	146.61575551988557
111	370.37	146.61575551988557
112	370.37	146.61575551988557
113	370.37	146.61575551988557
114	370.37	146.61575551988557
115	370.37	146.61575551988557
116	370.37	146.61575551988557
117	370.37	146.61575551988557
118	370.37	146.61575551988557
119	370.37	146.61575551988557
120	370.37	146.61575551988557
121	370.37	146.61575551988557
122	370.37	146.61575551988557
123	370.37	146.61575551988557
124	370.37	146.61575551988557
125	370.37	146.61575551988557
126	370.37	146.61575551988557
127	370.37	146.61575551988557
128	370.37	146.61575551988557
129	370.37	146.61575551988557
130	370.37	146.61575551988557
131	370.37	146.61575551988557
132	370.37	146.61575551988557
133	370.37	146.61575551988557
134	370.37	146.61575551988557
135	370.37	146.61575551988557
136	370.37	146.61575551988557
137	370.37	146.61575551988557
138	370.37	146.61575551988557
139	370.37	146.61575551988557
140	370.37	146.61575551988557
141	370.37	146.61575551988557
142	370.37	146.61575551988557
143	370.37	146.61575551988557
144	370.37	146.61575551988557
145	370.37	146.61575551988557
146	370.37	146.61575551988557
147	370.37	146.61575551988557
148	370.37	146.61575551988557
149	370.37	146.61575551988557
150	370.37	146.61575551988557
151	370.37	146.61575551988557
152	370.37	146.61575551988557
153	370.37	146.61575551988557
154	370.37	146.61575551988557
155	370.37	146.61575551988557
156	370.37	146.61575551988557
157	370.37	146.61575551988557
158	370.37	146.61575551988557
159	370.37	146.61575551988557
160	370.37	146.61575551988557
161	370.37	146.61575551988557
162	370.37	146.61575551988557
163	370.37	146.61575551988557
164	370.37	146.61575551988557
165	370.37	146.61575551988557
166	370.37	146.61575551988557
167	370.37	146.61575551988557
168	370.37	146.61575551988557
169	370.37	146.61575551988557
170	370.37	146.61575551988557
171	370.37	146.61575551988557
172	370.37	146.61575551988557
173	370.37	146.61575551988557
174	370.37	146.61575551988557
175	370.37	146.61575551988557
176	370.37	146.61575551988557
177	370.37	146.61575551988557
178	370.37	146.61575551988557
179	370.37	146.61575551988557
180	370.37	146.61575551988557
181	370.37	146.61575551988557
182	370.37	146.61575551988557
183	370.37	146.61575551988557
184	370.37	146.61575551988557
185	370.37	146.61575551988557
186	370.37	146.61575551988557
187	370.37	146.61575551988557
188	370.37	146.61575551988557
189	370.37	146.61575551988557
190	370.37	146.61575551988557
191	370.37	146.61575551988557
192	370.37	146.61575551988557
193	370.37	146.61575551988557
194	370.37	146.61575551988557
195	370.37	146.61575551988557
196	370.37	146.61575551988557
197	370.37	146.61575551988557
198	370.37	146.61575551988557
199	370.37	146.61575551988557
200	370.37	146.61575551988557
201	370.37	146.61575551988557
202	370.37	146.61575551988557
203	370.37	146.61575551988557
204	370.37	146.61575551988557
205	370.37	146.61575551988557
206	370.37	146.61575551988557
207	370.37	146.61575551988557
208	370.37	146.61575551988557
209	370.37	146.61575551988557
210	370.37	146.61575551988557
211	370.37	146.61575551988557
212	370.37	146.61575551988557
213	370.37	146.61575551988557
214	370.37	146.61575551988557
215	370.37	146.61575551988557
216	370.37	146.61575551988557
217	370.37	146.61575551988557
218	370.37	146.61575551988557
219	370.37	146.61575551988557
220	370.37	146.61575551988557
221	370.37	146.61575551988557
222	370.37	146.61575551988557
223	370.37	146.61575551988557
224	370.37	146.61575551988557
225	370.37	146.61575551988557
226	370.37	146.61575551988557
227	370.37	146.61575551988557
228	370.37	146.61575551988557
229	370.37	146.61575551988557
230	370.37	146.61575551988557
231	370.37	146.61575551988557
232	370.37	146.61575551988557
233	370.37	146.61575551988557
234	370.37	146.61575551988557
235	370.37	146.61575551988557
236	370.37	146.61575551988557
237	370.37	146.61575551988557
238	370.37	146.61575551988557
239	370.37	146.61575551988557
240	370.37	146.61575551988557
241	370.37	146.61575551988557
242	370.37	146.61575551988557
243	370.37	146.61575551988557
244	370.37	146.61575551988557
245	370.37	146.61575551988557
246	370.37	146.61575551988557
247	370.37	146.61575551988557
248	370.37	146.61575551988557
249	370.37	146.61575551988557
250	370.37	146.61575551988557
251	370.37	146.61575551988557
252	370.37	146.61575551988557
253	370.37	146.61575551988557
254	370.37	146.61575551988557
255	370.37	146.61575551988557
256	370.37	146.61575551988557
257	370.37	146.61575551988557
258	370.37	146.61575551988557
259	370.37	146.61575551988557
260	370.37	146.61575551988557
261	370.37	146.61575551988557
262	370.37	146.61575551988557
263	370.37	146.61575551988557
264	370.37	146.61575551988557
265	370.37	146.61575551988557
266	370.37	146.61575551988557
267	370.37	146.61575551988557
268	370.37	146.61575551988557
269	370.37	146.61575551988557
270	370.37	146.61575551988557
271	370.37	146.61575551988557
272	370.37	146.61575551988557
273	370.37	146.61575551988557
274	370.37	146.61575551988557
275	370.37	146.61575551988557
276	370.37	146.61575551988557
277	370.37	146.61575551988557
278	370.37	146.61575551988557
279	370.37	146.61575551988557
280	370.37	146.61575551988557
281	370.37	146.61575551988557
282	370.37	146.61575551988557
283	370.37	146.61575551988557
284	370.37	146.61575551988557
285	370.37	146.61575551988557
286	370.37	146.61575551988557
287	370.37	146.61575551988557
288	370.37	146.61575551988557
289	370.37	146.61575551988557
290	370.37	146.61575551988557
291	370.37	146.61575551988557
292	370.37	146.61575551988557
293	370.37	146.61575551988557
294	370.37	146.61575551988557
295	370.37	146.61575551988557
296	370.37	146.61575551988557
297	370.37	146.61575551988557
298	370.37	146.61575551988557
299	370.37	146.61575551988557
