# Supplementary material for: Task-Guided IRL in POMDPs that Scales
Source: arXiv:2301.01219 source file (2022-12-30)
Supplement: Supplementary file 14 [file obstacle_mem5_trajsize10pomdp_irl_si.tex]

% $\mathrm{Guided \ policy, \ |n|=10}$
x	y	err
0	0.0	0.0
1	-5.0	0.0
2	-9.996666666666666	0.12905640455071404
3	-13.141666666666667	30.523842001876154
4	-14.585	52.05480549382391
5	-12.121666666666666	79.79958352369701
6	-6.386666666666667	107.05696531390383
7	3.1566666666666667	134.26045132089166
8	13.18	156.31017539921672
9	21.506666666666668	172.72216598404913
10	28.651666666666667	185.79322825088852
11	35.19	196.76808828330968
12	39.08166666666666	204.57948332426457
13	43.626666666666665	212.20955984330914
14	49.461666666666666	220.03484996068286
15	59.123333333333335	229.19485477548847
16	69.095	237.3926900903511
17	84.75333333333333	246.55490765524934
18	106.16	255.26555662681415
19	131.01	261.6732948417401
20	156.47166666666666	264.8769384649335
21	180.02333333333334	265.1116421224989
22	205.17666666666668	262.17930020418487
23	228.075	256.8140430512542
24	248.69166666666666	249.60975527922943
25	268.01166666666666	240.5353505493315
26	281.6433333333333	232.8324851094072
27	297.10333333333335	222.10540138011524
28	308.685	212.77682935022221
29	319.0416666666667	203.20434689548736
30	327.8233333333333	194.0361533036784
31	336.19166666666666	184.16746436478934
32	343.3016666666667	174.78598531887118
33	346.95	169.6525788191834
34	350.4683333333333	164.32063878452882
35	353.68666666666667	159.08511921470065
36	356.6016666666667	154.00571308847256
37	358.0316666666667	151.43111964593743
38	360.8233333333333	145.97444567077122
39	361.96	143.66114668436424
40	362.77166666666665	141.9524903992725
41	363.08666666666664	141.28914497897057
42	363.91	139.43891816849353
43	363.9	139.48024949791545
44	363.89	139.5219262338355
45	364.04833333333335	139.15753422131158
46	364.545	137.94733768724984
47	364.71	137.53756783754335
48	364.87666666666667	137.11303653879506
49	364.87666666666667	137.11303653879506
50	364.87666666666667	137.11303653879506
51	364.87666666666667	137.11303653879506
52	364.87666666666667	137.11303653879506
53	364.87666666666667	137.11303653879506
54	364.87666666666667	137.11303653879506
55	364.87666666666667	137.11303653879506
56	364.87666666666667	137.11303653879506
57	364.87666666666667	137.11303653879506
58	364.87666666666667	137.11303653879506
59	364.87666666666667	137.11303653879506
60	364.87666666666667	137.11303653879506
61	364.87666666666667	137.11303653879506
62	364.87666666666667	137.11303653879506
63	364.87666666666667	137.11303653879506
64	364.87666666666667	137.11303653879506
65	364.87666666666667	137.11303653879506
66	364.87666666666667	137.11303653879506
67	364.87666666666667	137.11303653879506
68	364.87666666666667	137.11303653879506
69	364.87666666666667	137.11303653879506
70	364.87666666666667	137.11303653879506
71	364.87666666666667	137.11303653879506
72	364.87666666666667	137.11303653879506
73	364.87666666666667	137.11303653879506
74	364.87666666666667	137.11303653879506
75	364.87666666666667	137.11303653879506
76	364.87666666666667	137.11303653879506
77	364.87666666666667	137.11303653879506
78	364.87666666666667	137.11303653879506
79	364.87666666666667	137.11303653879506
80	364.87666666666667	137.11303653879506
81	364.87666666666667	137.11303653879506
82	364.87666666666667	137.11303653879506
83	364.87666666666667	137.11303653879506
84	364.87666666666667	137.11303653879506
85	364.87666666666667	137.11303653879506
86	364.87666666666667	137.11303653879506
87	364.87666666666667	137.11303653879506
88	364.87666666666667	137.11303653879506
89	364.87666666666667	137.11303653879506
90	364.87666666666667	137.11303653879506
91	364.87666666666667	137.11303653879506
92	364.87666666666667	137.11303653879506
93	364.87666666666667	137.11303653879506
94	364.87666666666667	137.11303653879506
95	364.87666666666667	137.11303653879506
96	364.87666666666667	137.11303653879506
97	364.87666666666667	137.11303653879506
98	364.87666666666667	137.11303653879506
99	364.87666666666667	137.11303653879506
100	364.87666666666667	137.11303653879506
101	364.87666666666667	137.11303653879506
102	364.87666666666667	137.11303653879506
103	364.87666666666667	137.11303653879506
104	364.87666666666667	137.11303653879506
105	364.87666666666667	137.11303653879506
106	364.87666666666667	137.11303653879506
107	364.87666666666667	137.11303653879506
108	364.87666666666667	137.11303653879506
109	364.87666666666667	137.11303653879506
110	364.87666666666667	137.11303653879506
111	364.87666666666667	137.11303653879506
112	364.87666666666667	137.11303653879506
113	364.87666666666667	137.11303653879506
114	364.87666666666667	137.11303653879506
115	364.87666666666667	137.11303653879506
116	364.87666666666667	137.11303653879506
117	364.87666666666667	137.11303653879506
118	364.87666666666667	137.11303653879506
119	364.87666666666667	137.11303653879506
120	364.87666666666667	137.11303653879506
121	364.87666666666667	137.11303653879506
122	364.87666666666667	137.11303653879506
123	364.87666666666667	137.11303653879506
124	364.87666666666667	137.11303653879506
125	364.87666666666667	137.11303653879506
126	364.87666666666667	137.11303653879506
127	364.87666666666667	137.11303653879506
128	364.87666666666667	137.11303653879506
129	364.87666666666667	137.11303653879506
130	364.87666666666667	137.11303653879506
131	364.87666666666667	137.11303653879506
132	364.87666666666667	137.11303653879506
133	364.87666666666667	137.11303653879506
134	364.87666666666667	137.11303653879506
135	364.87666666666667	137.11303653879506
136	364.87666666666667	137.11303653879506
137	364.87666666666667	137.11303653879506
138	364.87666666666667	137.11303653879506
139	364.87666666666667	137.11303653879506
140	364.87666666666667	137.11303653879506
141	364.87666666666667	137.11303653879506
142	364.87666666666667	137.11303653879506
143	364.87666666666667	137.11303653879506
144	364.87666666666667	137.11303653879506
145	364.87666666666667	137.11303653879506
146	364.87666666666667	137.11303653879506
147	364.87666666666667	137.11303653879506
148	364.87666666666667	137.11303653879506
149	364.87666666666667	137.11303653879506
150	364.87666666666667	137.11303653879506
151	364.87666666666667	137.11303653879506
152	364.87666666666667	137.11303653879506
153	364.87666666666667	137.11303653879506
154	364.87666666666667	137.11303653879506
155	364.87666666666667	137.11303653879506
156	364.87666666666667	137.11303653879506
157	364.87666666666667	137.11303653879506
158	364.87666666666667	137.11303653879506
159	364.87666666666667	137.11303653879506
160	364.87666666666667	137.11303653879506
161	364.87666666666667	137.11303653879506
162	364.87666666666667	137.11303653879506
163	364.87666666666667	137.11303653879506
164	364.87666666666667	137.11303653879506
165	364.87666666666667	137.11303653879506
166	364.87666666666667	137.11303653879506
167	364.87666666666667	137.11303653879506
168	364.87666666666667	137.11303653879506
169	364.87666666666667	137.11303653879506
170	364.87666666666667	137.11303653879506
171	364.87666666666667	137.11303653879506
172	364.87666666666667	137.11303653879506
173	364.87666666666667	137.11303653879506
174	364.87666666666667	137.11303653879506
175	364.87666666666667	137.11303653879506
176	364.87666666666667	137.11303653879506
177	364.87666666666667	137.11303653879506
178	364.87666666666667	137.11303653879506
179	364.87666666666667	137.11303653879506
180	364.87666666666667	137.11303653879506
181	364.87666666666667	137.11303653879506
182	364.87666666666667	137.11303653879506
183	364.87666666666667	137.11303653879506
184	364.87666666666667	137.11303653879506
185	364.87666666666667	137.11303653879506
186	364.87666666666667	137.11303653879506
187	364.87666666666667	137.11303653879506
188	364.87666666666667	137.11303653879506
189	364.87666666666667	137.11303653879506
190	364.87666666666667	137.11303653879506
191	364.87666666666667	137.11303653879506
192	364.87666666666667	137.11303653879506
193	364.87666666666667	137.11303653879506
194	364.87666666666667	137.11303653879506
195	364.87666666666667	137.11303653879506
196	364.87666666666667	137.11303653879506
197	364.87666666666667	137.11303653879506
198	364.87666666666667	137.11303653879506
199	364.87666666666667	137.11303653879506
200	364.87666666666667	137.11303653879506
201	364.87666666666667	137.11303653879506
202	364.87666666666667	137.11303653879506
203	364.87666666666667	137.11303653879506
204	364.87666666666667	137.11303653879506
205	364.87666666666667	137.11303653879506
206	364.87666666666667	137.11303653879506
207	364.87666666666667	137.11303653879506
208	364.87666666666667	137.11303653879506
209	364.87666666666667	137.11303653879506
210	364.87666666666667	137.11303653879506
211	364.87666666666667	137.11303653879506
212	364.87666666666667	137.11303653879506
213	364.87666666666667	137.11303653879506
214	364.87666666666667	137.11303653879506
215	364.87666666666667	137.11303653879506
216	364.87666666666667	137.11303653879506
217	364.87666666666667	137.11303653879506
218	364.87666666666667	137.11303653879506
219	364.87666666666667	137.11303653879506
220	364.87666666666667	137.11303653879506
221	364.87666666666667	137.11303653879506
222	364.87666666666667	137.11303653879506
223	364.87666666666667	137.11303653879506
224	364.87666666666667	137.11303653879506
225	364.87666666666667	137.11303653879506
226	364.87666666666667	137.11303653879506
227	364.87666666666667	137.11303653879506
228	364.87666666666667	137.11303653879506
229	364.87666666666667	137.11303653879506
230	364.87666666666667	137.11303653879506
231	364.87666666666667	137.11303653879506
232	364.87666666666667	137.11303653879506
233	364.87666666666667	137.11303653879506
234	364.87666666666667	137.11303653879506
235	364.87666666666667	137.11303653879506
236	364.87666666666667	137.11303653879506
237	364.87666666666667	137.11303653879506
238	364.87666666666667	137.11303653879506
239	364.87666666666667	137.11303653879506
240	364.87666666666667	137.11303653879506
241	364.87666666666667	137.11303653879506
242	364.87666666666667	137.11303653879506
243	364.87666666666667	137.11303653879506
244	364.87666666666667	137.11303653879506
245	364.87666666666667	137.11303653879506
246	364.87666666666667	137.11303653879506
247	364.87666666666667	137.11303653879506
248	364.87666666666667	137.11303653879506
249	364.87666666666667	137.11303653879506
250	364.87666666666667	137.11303653879506
251	364.87666666666667	137.11303653879506
252	364.87666666666667	137.11303653879506
253	364.87666666666667	137.11303653879506
254	364.87666666666667	137.11303653879506
255	364.87666666666667	137.11303653879506
256	364.87666666666667	137.11303653879506
257	364.87666666666667	137.11303653879506
258	364.87666666666667	137.11303653879506
259	364.87666666666667	137.11303653879506
260	364.87666666666667	137.11303653879506
261	364.87666666666667	137.11303653879506
262	364.87666666666667	137.11303653879506
263	364.87666666666667	137.11303653879506
264	364.87666666666667	137.11303653879506
265	364.87666666666667	137.11303653879506
266	364.87666666666667	137.11303653879506
267	364.87666666666667	137.11303653879506
268	364.87666666666667	137.11303653879506
269	364.87666666666667	137.11303653879506
270	364.87666666666667	137.11303653879506
271	364.87666666666667	137.11303653879506
272	364.87666666666667	137.11303653879506
273	364.87666666666667	137.11303653879506
274	364.87666666666667	137.11303653879506
275	364.87666666666667	137.11303653879506
276	364.87666666666667	137.11303653879506
277	364.87666666666667	137.11303653879506
278	364.87666666666667	137.11303653879506
279	364.87666666666667	137.11303653879506
280	364.87666666666667	137.11303653879506
281	364.87666666666667	137.11303653879506
282	364.87666666666667	137.11303653879506
283	364.87666666666667	137.11303653879506
284	364.87666666666667	137.11303653879506
285	364.87666666666667	137.11303653879506
286	364.87666666666667	137.11303653879506
287	364.87666666666667	137.11303653879506
288	364.87666666666667	137.11303653879506
289	364.87666666666667	137.11303653879506
290	364.87666666666667	137.11303653879506
291	364.87666666666667	137.11303653879506
292	364.87666666666667	137.11303653879506
293	364.87666666666667	137.11303653879506
294	364.87666666666667	137.11303653879506
295	364.87666666666667	137.11303653879506
296	364.87666666666667	137.11303653879506
297	364.87666666666667	137.11303653879506
298	364.87666666666667	137.11303653879506
299	364.87666666666667	137.11303653879506
