# Supplementary material for: Task-Guided IRL in POMDPs that Scales
Source: arXiv:2301.01219 source file (2022-12-30)
Supplement: Supplementary file 15 [file rock_mem10_trajsize10mdp_irl_si.tex]

% $\mathrm{Guided \ policy, \ |n|=10}$
x	y	err
0	0.0	0.0
1	-0.09999999999999991	9.71445146547012e-17
2	-0.19999999999999982	1.942890293094024e-16
3	-0.46759999999997715	0.8126193696928586
4	-2.2514333333333214	2.2077057349706437
5	-3.288933333333277	3.95722009271945
6	-4.125099999999959	5.549025138706824
7	-3.598633333333282	10.582543556830833
8	0.0204666666666761	21.130115343956156
9	18.066066666665947	38.464586074234944
10	23.186899999999223	40.894817907937764
11	24.87949999999931	41.688674917975725
12	27.343299999999378	42.82281504575945
13	28.438933333332724	43.25847143464736
14	29.53619999999943	43.729181594140435
15	30.499599999999457	44.0993644682854
16	31.563133333332775	44.52867114772495
17	32.49313333333277	44.84479530761825
18	33.92363333333276	45.328786197428464
19	34.82103333333279	45.5799200043055
20	36.052166666666096	45.92899645437073
21	36.849766666666106	46.12405807470686
22	37.6810666666661	46.32077749990295
23	38.34573333333275	46.441874084302825
24	39.27736666666608	46.647118357574215
25	39.97549999999943	46.763072715017735
26	40.50579999999943	46.8560662706541
27	41.103766666666104	46.93318977524191
28	41.9018999999994	47.05490516113398
29	42.332833333332744	47.103859983079644
30	43.197399999999405	47.2074558366935
31	43.928399999999435	47.259402310792005
32	44.691566666666155	47.33353616143111
33	45.522766666666236	47.37706475724555
34	46.28733333333297	47.40353150932501
35	46.91833333333298	47.41199978791085
36	47.81619999999968	47.43229178762784
37	48.547299999999694	47.4187566901888
38	49.34516666666641	47.40283876842845
39	50.1761333333331	47.376063756383196
40	50.87376666666645	47.34461034245526
41	51.67009999999977	47.28268022567386
42	52.73489999999986	47.201662032779055
43	53.36489999999987	47.13356056276017
44	54.12996666666657	47.03563548345253
45	54.76173333333328	46.94927144264892
46	55.42703333333325	46.85548732573611
47	55.758499999999906	46.80185588645731
48	56.39003333333321	46.71084810475576
49	57.11996666666652	46.576766432763165
50	57.75159999999989	46.45521776334719
51	58.31659999999985	46.31617209758737
52	59.21526666666653	46.1023199733901
53	59.54666666666654	46.02396805530341
54	60.04493333333318	45.904364581836774
55	60.77633333333326	45.7066895894048
56	61.541466666666615	45.49004814809023
57	62.00653333333324	45.34737622673281
58	62.73859999999993	45.123844362376786
59	63.27083333333327	44.943278911373774
60	63.669566666666604	44.817067252839585
61	64.0013666666666	44.690651238622436
62	64.43339999999992	44.545702573574026
63	65.09896666666656	44.270733925083626
64	65.5646333333332	44.097817094865796
65	65.7967333333332	44.00083759803758
66	66.26229999999984	43.80727552256604
67	66.69469999999981	43.61786570405159
68	67.0603666666665	43.46279565174754
69	67.42589999999983	43.28818421374717
70	67.65809999999979	43.18254949695133
71	68.19046666666647	42.92910491863943
72	68.5895999999998	42.743707667600916
73	68.9216333333331	42.57505570948252
74	69.15359999999977	42.46957013015306
75	69.58559999999976	42.25769767320499
76	70.28479999999972	41.901454576502225
77	70.6172666666664	41.72236500801708
78	70.98333333333308	41.528493297440164
79	71.1824666666664	41.41884497724302
80	71.51516666666639	41.23631344626824
81	71.64763333333305	41.162827742177896
82	72.04689999999971	40.94544057307662
83	72.27929999999972	40.800448382054405
84	72.61183333333307	40.609916727800865
85	72.87749999999971	40.44777930142382
86	73.24323333333305	40.22767042155878
87	73.47533333333303	40.077371398611334
88	73.94116666666633	39.79171850991409
89	74.27359999999963	39.565198550915
90	74.70619999999964	39.28323393289695
91	74.77173333333295	39.23851077273752
92	75.23739999999961	38.92451551280637
93	75.50299999999959	38.734039521674624
94	75.9021333333329	38.449002181880076
95	76.30129999999954	38.150072367472006
96	76.56716666666621	37.95158369957099
97	76.83309999999955	37.74297075028247
98	77.06573333333287	37.56647325025579
99	77.36506666666618	37.31963754283906
100	77.56446666666615	37.166620562662345
101	77.89719999999947	36.905352622079064
102	78.0300333333328	36.799277094333156
103	78.22949999999946	36.64067047808137
104	78.46223333333279	36.45720327103533
105	78.62823333333276	36.32511508876755
106	78.76073333333275	36.219314434827346
107	79.09333333333272	35.9138695894623
108	79.42596666666603	35.62172093539103
109	79.65846666666603	35.410290241428726
110	79.82429999999935	35.26912690786898
111	80.1569333333327	34.960428753028275
112	80.58986666666603	34.56376306647698
113	80.65593333333267	34.49699877953966
114	80.88879999999934	34.28138408174337
115	81.05476666666598	34.11721604428234
116	81.32089999999931	33.8569362640805
117	81.35353333333262	33.827290178920514
118	81.75309999999928	33.44182815562005
119	81.88573333333262	33.30607566889577
120	82.11849999999929	33.066232338797
121	82.25116666666592	32.923116680718834
122	82.5840666666659	32.57985481033036
123	82.68353333333256	32.470763087977545
124	82.98316666666587	32.144355024984165
125	83.01606666666585	32.10638558286413
126	83.28249999999919	31.817093787512103
127	83.38209999999918	31.702403845607762
128	83.44829999999916	31.62762174286944
129	83.58109999999917	31.47643615134992
130	83.78063333333249	31.25486258060059
131	83.91349999999915	31.103479994206385
132	84.14649999999915	30.8392051521542
133	84.2460666666658	30.722708721653465
134	84.37903333333246	30.5718468049538
135	84.51193333333244	30.406246138946823
136	84.6782999999991	30.21357232177841
137	84.71116666666576	30.17583247079617
138	84.94423333333242	29.89226600218753
139	85.07726666666574	29.725122425240524
140	85.17703333333242	29.60537083929603
141	85.21006666666574	29.56130339924504
142	85.37646666666575	29.359037101300842
143	85.44276666666575	29.26868316726162
144	85.50906666666573	29.182697118821874
145	85.67539999999904	28.96233257480005
146	85.8417666666657	28.75326043330636
147	85.90803333333236	28.66513827163946
148	86.07426666666568	28.443563849528882
149	86.14043333333233	28.354021263521425
150	86.30673333333233	28.132926047525764
151	86.506499999999	27.849481043937864
152	86.63966666666566	27.66135559263564
153	86.67273333333232	27.612330033197708
154	86.73913333333232	27.522971410239837
155	86.87076666666563	27.337136196248082
156	86.97053333333228	27.195385730834918
157	87.03696666666562	27.104046748266605
158	87.20349999999894	26.871289965624197
159	87.20333333333228	26.871838956217807
160	87.30313333333227	26.731268148909184
161	87.33613333333227	26.67993067923684
162	87.43586666666562	26.53329179695234
163	87.50219999999895	26.438334450062342
164	87.66863333333228	26.18686705454078
165	87.76846666666565	26.041087515352384
166	87.83499999999898	25.94305497944788
167	87.93486666666566	25.784271516738613
168	87.93466666666563	25.784962249773294
169	87.9677333333323	25.735868851252842
170	88.1008333333323	25.530523221669576
171	88.16729999999897	25.43014721500178
172	88.23379999999898	25.328824638344557
173	88.33369999999898	25.164471535149232
174	88.36689999999899	25.113311896083864
175	88.43343333333232	25.004718998865595
176	88.46656666666566	24.947986937070258
177	88.49956666666566	24.891418396954034
178	88.56596666666564	24.78735050515771
179	88.69899999999897	24.571347656704635
180	88.83213333333231	24.357542174493016
181	88.83179999999898	24.35877519006257
182	88.9982333333323	24.08223633466953
183	89.03136666666563	24.022409249120198
184	89.16463333333229	23.80131325226059
185	89.23119999999898	23.67842153860749
186	89.23099999999897	23.679190280356753
187	89.26416666666562	23.623815934466933
188	89.36406666666562	23.4486749191126
189	89.4305666666656	23.329614420564468
190	89.46369999999895	23.26737900244327
191	89.53009999999892	23.153542075817686
192	89.59656666666562	23.03840196018133
193	89.66299999999896	22.910682464736617
194	89.79616666666561	22.675424185056134
195	89.82926666666562	22.61701712123454
196	89.89566666666563	22.49852783085044
197	89.99546666666565	22.31857073042281
198	90.09536666666567	22.123777597844548
199	90.16193333333234	21.988083687811876
200	90.19513333333234	21.926727898059582
201	90.19499999999901	21.927279090971176
202	90.26153333333234	21.803347609535336
203	90.32803333333236	21.678950408146868
204	90.32783333333235	21.679788174831522
205	90.39436666666568	21.55402464194479
206	90.49433333333235	21.36289262300919
207	90.52759999999901	21.29877691887484
208	90.52749999999901	21.299203750766747
209	90.56076666666567	21.23515805008837
210	90.59406666666567	21.170565528477486
211	90.62729999999902	21.106167930488745
212	90.62716666666567	21.106749599094808
213	90.62703333333234	21.10733188252099
214	90.72696666666566	20.911163433253137
215	90.760199999999	20.839042267500368
216	90.75999999999902	20.839930102250175
217	90.79303333333237	20.768393810440898
218	90.85946666666568	20.636032492920947
219	91.02599999999902	20.29227054816708
220	91.09253333333234	20.14859989136258
221	91.09239999999899	20.149206326139417
222	91.15889999999901	20.011457904327322
223	91.22539999999901	19.872196192335384
224	91.22523333333233	19.87298618591492
225	91.35846666666569	19.56960470514316
226	91.39169999999902	19.498454326176834
227	91.42493333333236	19.427158266943856
228	91.45819999999902	19.355212203090442
229	91.49146666666569	19.275844309624677
230	91.52473333333236	19.203208454028793
231	91.55796666666569	19.1305733456219
232	91.55779999999902	19.13137490685566
233	91.6243666666657	18.984619817075203
234	91.69099999999904	18.83580594683094
235	91.72419999999904	18.761269707209564
236	91.72399999999905	18.762281062457717
237	91.75716666666571	18.687937160252602
238	91.85706666666572	18.45256396084013
239	91.92369999999906	18.276346142213413
240	91.92366666666571	18.27652227737984
241	91.95699999999906	18.19125919226011
242	91.95689999999905	18.191781451798278
243	91.95679999999906	18.192304245476738
244	91.95669999999905	18.192827573249687
245	92.05666666666573	17.942235708579265
246	92.05663333333241	17.942408311006773
247	92.05653333333241	17.94293966946977
248	92.08979999999907	17.863102267710005
249	92.08969999999908	17.863635797619743
250	92.15629999999908	17.68838678276425
251	92.15626666666576	17.688569022456917
252	92.15623333333241	17.688751448653026
253	92.18953333333242	17.60037605040184
254	92.18949999999907	17.60055149940849
255	92.18946666666574	17.6007271359893
256	92.22279999999908	17.519470696722834
257	92.2227333333324	17.519830950351377
258	92.22266666666573	17.520191576831674
259	92.22253333333241	17.520904816310708
260	92.28913333333242	17.349361810997056
261	92.28903333333241	17.34989653376145
262	92.35566666666577	17.184356681457512
263	92.35563333333245	17.1845368941252
264	92.38896666666577	17.100979161017257
265	92.38896666666577	17.100979161017257
266	92.38889999999911	17.101340301957034
267	92.3887999999991	17.101882583310523
268	92.42206666666578	17.01860961013608
269	92.45523333333244	16.935221264538875
270	92.48843333333244	16.850973944519726
271	92.52163333333243	16.75807632154992
272	92.62156666666577	16.498832429767692
273	92.6213999999991	16.499788949357345
274	92.65453333333244	16.41337359540176
275	92.6876999999991	16.317862769881224
276	92.82099999999913	15.942751090490411
277	92.85433333333246	15.843046883587881
278	92.85433333333246	15.843046883587881
279	92.85429999999911	15.843242981683698
280	92.8542666666658	15.843439287674546
281	92.88756666666579	15.752123309114658
282	92.88753333333247	15.752320821037477
283	92.92076666666578	15.660808368202497
284	92.92063333333245	15.66162031630891
285	92.92046666666576	15.662631572702555
286	93.02036666666577	15.373890481339636
287	93.05363333333244	15.270454701772813
288	93.08693333333244	15.17504363295913
289	93.12019999999912	15.070095287024499
290	93.12013333333245	15.070518061728594
291	93.12006666666578	15.07094126663059
292	93.1866666666658	14.867601764313703
293	93.18659999999912	14.868031491760942
294	93.25323333333246	14.660907755395746
295	93.25319999999913	14.661130121060399
296	93.25316666666579	14.66135271063205
