# Supplementary material for: Task-Guided IRL in POMDPs that Scales
Source: arXiv:2301.01219 source file (2022-12-30)
Supplement: Supplementary file 18 [file rock_mem1_trajsize10pomdp_irl_si.tex]

% $\mathrm{Guided \ policy, \ |n|=1}$
x	y	err
0	0.0	0.0
1	-0.09999999999999991	9.71445146547012e-17
2	-0.20133333333333345	0.07301750170716093
3	-0.25389999999999496	2.6006316136662813
4	-0.5673333333333507	5.337859704246889
5	-0.7951333333333412	7.573977135487536
6	-0.7918333333333066	10.32644711274016
7	1.4814666666667535	19.307668507155867
8	9.610766666666876	33.420567530772225
9	18.300433333332766	41.825686722542116
10	27.010499999999997	47.0802850432118
11	34.24333333333267	49.86527905823419
12	40.36256666666723	51.242439657757316
13	45.46223333333273	51.780267383874516
14	50.18940000000076	51.730046275254864
15	53.355333333333355	51.44611366814394
16	57.062199999998874	50.871921834740405
17	60.10039999999911	50.10007950599151
18	62.745033333333616	49.23251393810388
19	64.60383333333405	48.548283752420566
20	66.74326666666663	47.60112023887196
21	68.37369999999905	46.796737190143325
22	70.45319999999904	45.59293749869582
23	72.21590000000019	44.42999516681654
24	73.20616666666719	43.80591290346046
25	74.67143333333328	42.7365929145686
26	75.94846666666598	41.75612295598743
27	76.99479999999923	40.865409818411
28	78.13536666666688	39.83990628166959
29	79.31176666666694	38.71630291680187
30	80.05829999999983	38.00200500556937
31	80.7604666666661	37.31534890339667
32	81.37379999999933	36.67822887708723
33	81.82230000000008	36.171526177966705
34	82.54210000000023	35.2248760242435
35	83.26539999999989	34.41882115219351
36	83.97089999999953	33.5095527154571
37	84.57676666666617	32.631978848141436
38	84.97903333333339	32.12709423107256
39	85.65153333333345	31.074830935161785
40	86.06036666666652	30.34227445658758
41	86.57376666666626	29.495712939547992
42	86.89153333333287	28.94926910388048
43	87.3470333333333	28.136801722990743
44	87.89096666666667	27.16365430249687
45	88.17666666666655	26.674128206101834
46	88.46509999999968	26.123320972967203
47	88.68189999999967	25.73508983968515
48	88.90163333333334	25.394778216506822
49	89.24826666666668	24.6224068075313
50	89.43516666666655	24.24045984104989
51	89.72359999999982	23.474427001313636
52	89.98299999999975	22.980113671027272
53	90.17320000000004	22.40469478539411
54	90.36236666666666	21.96094670998701
55	90.45563333333327	21.64215827805134
56	90.64763333333322	21.028778401646502
57	90.77179999999986	20.64915829019033
58	90.92823333333334	20.263579304067253
59	91.0541666666666	19.98237079625174
60	91.1106999999999	19.839864133691435
61	91.16999999999985	19.67068970151599
62	91.29343333333316	19.405022035860235
63	91.41963333333331	19.094991084895103
64	91.48193333333329	18.85674787078155
65	91.60703333333325	18.549678538065333
66	91.73486666666655	17.982633779535334
67	91.76539999999983	17.794028478865197
68	91.796	17.71233122243743
69	91.85866666666662	17.537127612265596
70	91.85606666666659	17.55599697716481
71	91.88409999999988	17.386399201387242
72	91.94829999999988	17.157939185986304
73	92.01383333333328	16.87098116013276
74	92.14479999999995	16.288436786874264
75	92.17579999999991	16.185605364850137
76	92.30826666666658	15.752124459753198
77	92.37409999999988	15.528602615496313
78	92.40529999999995	15.435602846773895
79	92.43653333333324	15.333209230802087
80	92.46919999999992	15.219857139934035
81	92.46846666666657	15.225364767898146
82	92.46639999999987	15.240210115786898
83	92.46566666666662	15.245728622214942
84	92.49833333333325	15.130803367817416
85	92.53103333333327	15.014467920383396
86	92.53036666666658	15.019620763040448
87	92.52839999999989	15.034046919353806
88	92.56109999999995	14.916250985306746
89	92.56049999999995	14.920999399615715
90	92.58923333333325	14.832749152204471
91	92.58733333333326	14.854520957906653
92	92.6200999999999	14.72475871867964
93	92.61819999999996	14.739122840024583
94	92.65103333333327	14.625587587018643
95	92.71733333333326	14.249903375890684
96	92.71689999999991	14.253573507136094
97	92.7164999999999	14.256987681484448
98	92.74939999999992	14.11892393114055
99	92.81569999999994	13.83363932027051
100	92.84869999999994	13.700012590383546
101	92.88173333333326	13.554148675917958
102	92.88146666666658	13.556677193012861
103	92.8811666666666	13.559470318030685
104	92.88089999999993	13.56201134996821
105	92.9139666666666	13.423252273532244
106	92.91369999999993	13.42581377955666
107	92.94546666666659	13.315033587974478
108	92.94393333333328	13.337695322989246
109	92.97706666666659	12.97020691413813
110	93.01023333333328	12.559288671957253
111	93.04343333333327	12.416498307180806
112	93.04329999999993	12.417660076546934
113	93.04316666666661	12.418822809438147
114	93.04303333333327	12.419986505583967
115	93.04293333333327	12.420870744928632
116	93.04279999999993	12.422036125101707
117	93.04266666666659	12.423202467783996
118	93.04253333333328	12.424369772704331
119	93.07576666666658	12.27747542231527
120	93.07566666666659	12.278374263539815
121	93.07423333333325	12.290905828249183
122	93.07413333333325	12.291816149328387
123	93.07403333333326	12.292727215670649
124	93.07393333333326	12.293639027110348
125	93.07383333333325	12.294551583481608
126	93.07373333333327	12.29546488461858
127	93.07363333333325	12.296378930355399
128	93.07219999999994	12.309850817942477
129	93.07209999999992	12.310776238320678
130	93.07203333333325	12.311393687646483
131	93.07193333333325	12.312320344363249
132	93.07183333333323	12.313247742664112
133	93.07173333333326	12.314175882381347
134	93.10499999999992	12.139534381515585
135	93.10493333333325	12.140163466591204
136	93.1048666666666	12.140793067817167
137	93.10483333333326	12.141097148619759
138	93.10476666666659	12.141727524487091
139	93.10469999999991	12.14235841630444
140	93.10463333333327	12.142989823991323
141	93.1045666666666	12.143621747467098
142	93.13786666666658	11.952693676136603
143	93.13783333333326	11.953004307379086
144	93.13779999999991	11.953315209318838
145	93.13776666666658	11.953626381934896
146	93.13773333333326	11.953937825205882
147	93.13769999999991	11.954249539110856
148	93.13766666666659	11.954561523628616
149	93.13763333333324	11.954873778737923
150	93.13759999999992	11.955186304417495
151	93.13756666666659	11.95549910064634
152	93.13753333333325	11.955812167403085
153	93.13749999999992	11.956125504666332
154	93.13746666666658	11.956439112415039
155	93.13746666666658	11.956439112415039
156	93.13743333333325	11.956752990627924
157	93.13739999999993	11.95706713928353
158	93.13736666666658	11.957381558360646
159	93.17069999999991	11.780861803931598
160	93.17069999999991	11.780861803931598
161	93.17069999999991	11.780861803931598
162	93.17069999999991	11.780861803931598
163	93.17069999999991	11.780861803931598
164	93.17069999999991	11.780861803931598
165	93.17069999999991	11.780861803931598
166	93.17069999999991	11.780861803931598
167	93.17069999999991	11.780861803931598
168	93.17069999999991	11.780861803931598
169	93.17069999999991	11.780861803931598
170	93.17069999999991	11.780861803931598
171	93.17069999999991	11.780861803931598
172	93.17069999999991	11.780861803931598
173	93.17069999999991	11.780861803931598
174	93.17069999999991	11.780861803931598
175	93.17069999999991	11.780861803931598
176	93.17069999999991	11.780861803931598
177	93.17069999999991	11.780861803931598
178	93.17069999999991	11.780861803931598
179	93.17069999999991	11.780861803931598
180	93.17069999999991	11.780861803931598
181	93.17069999999991	11.780861803931598
182	93.17069999999991	11.780861803931598
183	93.17069999999991	11.780861803931598
184	93.17069999999991	11.780861803931598
185	93.17069999999991	11.780861803931598
186	93.17069999999991	11.780861803931598
187	93.17069999999991	11.780861803931598
188	93.17069999999991	11.780861803931598
189	93.17069999999991	11.780861803931598
190	93.17069999999991	11.780861803931598
191	93.17069999999991	11.780861803931598
192	93.17069999999991	11.780861803931598
193	93.17069999999991	11.780861803931598
194	93.17069999999991	11.780861803931598
195	93.17069999999991	11.780861803931598
196	93.17069999999991	11.780861803931598
197	93.17069999999991	11.780861803931598
198	93.17069999999991	11.780861803931598
199	93.17069999999991	11.780861803931598
200	93.17069999999991	11.780861803931598
201	93.17069999999991	11.780861803931598
202	93.17069999999991	11.780861803931598
203	93.17069999999991	11.780861803931598
204	93.17069999999991	11.780861803931598
205	93.17069999999991	11.780861803931598
206	93.17069999999991	11.780861803931598
207	93.17069999999991	11.780861803931598
208	93.17069999999991	11.780861803931598
209	93.17069999999991	11.780861803931598
210	93.17069999999991	11.780861803931598
211	93.17069999999991	11.780861803931598
212	93.17069999999991	11.780861803931598
213	93.17069999999991	11.780861803931598
214	93.17069999999991	11.780861803931598
215	93.17069999999991	11.780861803931598
216	93.17069999999991	11.780861803931598
217	93.17069999999991	11.780861803931598
218	93.17069999999991	11.780861803931598
219	93.17069999999991	11.780861803931598
220	93.17069999999991	11.780861803931598
221	93.17069999999991	11.780861803931598
222	93.17069999999991	11.780861803931598
223	93.17069999999991	11.780861803931598
224	93.17069999999991	11.780861803931598
225	93.17069999999991	11.780861803931598
226	93.17069999999991	11.780861803931598
227	93.17069999999991	11.780861803931598
228	93.17069999999991	11.780861803931598
229	93.17069999999991	11.780861803931598
230	93.17069999999991	11.780861803931598
231	93.17069999999991	11.780861803931598
232	93.17069999999991	11.780861803931598
233	93.17069999999991	11.780861803931598
234	93.17069999999991	11.780861803931598
235	93.17069999999991	11.780861803931598
236	93.17069999999991	11.780861803931598
237	93.17069999999991	11.780861803931598
238	93.17069999999991	11.780861803931598
239	93.17069999999991	11.780861803931598
240	93.17069999999991	11.780861803931598
241	93.17069999999991	11.780861803931598
242	93.17069999999991	11.780861803931598
243	93.17069999999991	11.780861803931598
244	93.17069999999991	11.780861803931598
245	93.17069999999991	11.780861803931598
246	93.17069999999991	11.780861803931598
247	93.17069999999991	11.780861803931598
248	93.17069999999991	11.780861803931598
249	93.17069999999991	11.780861803931598
250	93.17069999999991	11.780861803931598
251	93.17069999999991	11.780861803931598
252	93.17069999999991	11.780861803931598
253	93.17069999999991	11.780861803931598
254	93.17069999999991	11.780861803931598
255	93.17069999999991	11.780861803931598
256	93.17069999999991	11.780861803931598
257	93.17069999999991	11.780861803931598
258	93.17069999999991	11.780861803931598
259	93.17069999999991	11.780861803931598
260	93.17069999999991	11.780861803931598
261	93.17069999999991	11.780861803931598
262	93.17069999999991	11.780861803931598
263	93.17069999999991	11.780861803931598
264	93.17069999999991	11.780861803931598
265	93.17069999999991	11.780861803931598
266	93.17069999999991	11.780861803931598
267	93.17069999999991	11.780861803931598
268	93.17069999999991	11.780861803931598
269	93.17069999999991	11.780861803931598
270	93.17069999999991	11.780861803931598
271	93.17069999999991	11.780861803931598
272	93.17069999999991	11.780861803931598
273	93.17069999999991	11.780861803931598
274	93.17069999999991	11.780861803931598
275	93.17069999999991	11.780861803931598
276	93.17069999999991	11.780861803931598
277	93.17069999999991	11.780861803931598
278	93.17069999999991	11.780861803931598
279	93.17069999999991	11.780861803931598
280	93.17069999999991	11.780861803931598
281	93.17069999999991	11.780861803931598
282	93.17069999999991	11.780861803931598
283	93.17069999999991	11.780861803931598
284	93.17069999999991	11.780861803931598
285	93.17069999999991	11.780861803931598
286	93.17069999999991	11.780861803931598
287	93.17069999999991	11.780861803931598
288	93.17069999999991	11.780861803931598
289	93.17069999999991	11.780861803931598
290	93.17069999999991	11.780861803931598
291	93.17069999999991	11.780861803931598
292	93.17069999999991	11.780861803931598
293	93.17069999999991	11.780861803931598
294	93.17069999999991	11.780861803931598
295	93.17069999999991	11.780861803931598
296	93.17069999999991	11.780861803931598
297	93.17069999999991	11.780861803931598
298	93.17069999999991	11.780861803931598
299	93.17069999999991	11.780861803931598
300	93.17069999999991	11.780861803931598
301	93.17069999999991	11.780861803931598
302	93.17069999999991	11.780861803931598
303	93.17069999999991	11.780861803931598
304	93.17069999999991	11.780861803931598
305	93.17069999999991	11.780861803931598
306	93.17069999999991	11.780861803931598
307	93.17069999999991	11.780861803931598
308	93.17069999999991	11.780861803931598
309	93.17069999999991	11.780861803931598
310	93.17069999999991	11.780861803931598
311	93.17069999999991	11.780861803931598
